# Supplementary material for: Billion-scale semi-supervised learning for image classification
Source: arXiv:1905.00546 source file (2019-05-02)
Supplement: Supplementary file 1 [file appendix.tex]

% !TEX root = self_training.tex

\section{Appendix}
This section records experiments results for different models. 
The quantitative results may show the trend of different experiment settings more clearly.

\subsection{Comparison with the state-of-the-art}

\subsubsection{ImageNet1K}

% WE SHOULD PUT ALL THESE INTO A PLOT LATER
\begin{table}[!ht]
\centering
\begin{tabular}{|c|c|c|c|c|}
\hline
Architecture       & Approach                  & top-1 & top-5 \\ \hline
ResNet-18          & Vanilla \cite{he2016deep} & 69.9  & 89.26 \\ \hline 
ResNet-50          & Vanilla \cite{he2016deep} & 76.45 & 93.22 \\ \hline 
ResNext-101-32x4   & Vanilla \cite{xie2017aggregated} & 78.48 & 94.18 \\ \hline
ResNext-101-32x8   & Vanilla \cite{xie2017aggregated} & 79.06  & 94.39 \\ \hline
ResNext-101-32x16  & Vanilla \cite{xie2017aggregated} & 79.59 & 94.65 \\ \hline
ResNext-101-32x48  & Vanilla \cite{xie2017aggregated} & 79.72 & 94.72 \\ \hline

ResNet-18  & LabelRefinery \cite{bagherinezhad2018label} & 72.52 (+2.8\%) &  - \\ \hline
ResNet-50  & LabelRefinery \cite{bagherinezhad2018label} & 76.5  (+0.8\%) &  - \\ \hline
ResNet-50  & AutoAugment   \cite{cubuk2018autoaugment}   & 77.63 (+2.33\%) & 93.82 (+0.74\%) \\ \hline

% \multirow{2}{*}{\begin{tabular}[c]{@{}c@{}}ResNet\\18\\(\%)\end{tabular}}  & \multirow{2}{*}{ \begin{tabular}[c]{@{}c@{}}Vanilla\\\cite{}\\(\%)\end{tabular}  } & \multirow{2}{*}{69.9} & \multirow{2}{*}{88.00}  \\ 
%             &  &  &  \\ \hline
%\multirow{2}{*}{ResNext-101 32x4d}  &  &  &  \\ \hline
\end{tabular}
\caption{Accuracy of various ImageNet1K models compared to the state of the art. The incremental gain is with respect to the reference paper's baseline implementation.
\rv{This table should go in the main paper, not in appendices}
}
\label{tab:vid}
\end{table}

\subsubsection{Kinetics}

\subsubsection{COCO}
